# Supplementary material for: InfoBatch: Lossless Training Speed Up by Unbiased Dynamic Data Pruning
Source: arXiv:2303.04947 source file (2023-10-20)
Supplement: Supplementary file 1 [file appendix.tex]

\section{Proof of Theorem 1}

We prove the \textbf{Theorem 1} which extends the learning theories of domain adaptation \citep{ben2010theory} for the black-box domain adaptation and provides theoretical justifications for our method.

Denote $\mathcal{X}_t\sim \mathcal{D}_T$ as the target domain with its sample distribution. $\mathcal{X}_e\sim \mathcal{D}_e$ and $\mathcal{X}_h\sim \mathcal{D}_h$ denote the easy-to-adapt clean subdomain and the hard-to-adapt noisy subdomain with their corresponding sample distributions, respectively. Denote $y_e,y_h$ and $\hat{y}_e,\hat{y}_h$ as the ground truth labels and the pseudo labels of $\mathcal{X}_e, \mathcal{X}_h$, respectively. Let $h$ denote a hypothesis. As our method performs training on a mixture of the clean set and the noisy set with pseudo labels, the error of our method can be formulated as a convex combination of the errors of the clean set and the noisy set:
\begin{equation}
    \epsilon_\alpha(h) = \alpha \epsilon_e(h,\hat{y}_e)+(1-\alpha)\epsilon_h(h,\hat{y}_h),
\end{equation}
where $\alpha$ is the trade-off hyper-parameter, and $\epsilon_e(h,\hat{y}_e),\epsilon_h(h,\hat{y}_h)$ represents the expected error of the easy-to-adapt clean set $\mathcal{X}_e$ and the hard-to-adapt noisy set $\mathcal{X}_h$, respectively, defined by
\begin{align}
    & \epsilon_e(h,\hat{y}_e)=\mathbb{E}_{x\sim \mathcal{D}_e} [|h(x)-\hat{y}_e|]\\
    & \epsilon_h(h,\hat{y}_h)=\mathbb{E}_{x\sim \mathcal{D}_h} [|h(x)-\hat{y}_h|].
\end{align}
We use the shorthand $\epsilon_e(h)=\epsilon_e(h,f_e)$ in the proof.

Then, we derive an upper bound of how the error $\epsilon_\alpha(h)$ is close to an oracle error of the target domain $\epsilon_t(h,y_t)$ where $y_t$ is the ground truth labels of the target domain, which is illustrated in \textbf{Theorem 1}:
\begin{theorem}
Let $h$ be a hypothesis in class $\mathcal{H}$. Then
\begin{equation}
|\epsilon_\alpha(h)-\epsilon_t(h,y_t)|\leq \alpha(d_{\mathcal{H}\triangle\mathcal{H}}(\mathcal{D}_e,\mathcal{D}_h)+\lambda+\hat{\lambda})+\rho_h,
\end{equation}
where the ideal risk is the combined error of the ideal joint hypothesis $\lambda=\epsilon_e(h^*)+\epsilon_h(h^*)$, the distribution discrepancy $d_\mathcal{\mathcal{H}\triangle\mathcal{H}}(\mathcal{D}_e,\mathcal{D}_h)=2\sup_{h,h' \in \mathcal{H}} |\mathbb{E}_{x\sim \mathcal{D}_e}[h(x)\ne h'(x)] - \mathbb{E}_{x\sim \mathcal{D}_h}[h(x)\ne h'(x)]|$, and $\rho_h$ denote the pseudo label rate of $\hat{y}_h$. The ideal joint hypothesis is given by $h^*=\arg \min_{h\in\mathcal{H}}(\epsilon_e(h)+\epsilon_h(h))$, deriving the ideal risk $\lambda=\epsilon_e(h^*)+\epsilon_h(h^*)$ and the pseudo risk $\hat{\lambda}=\epsilon_e(h^*,\hat{y}_e)+\epsilon_h(h^*,\hat{y}_h)$.
\end{theorem}

\textit{Proof:}
\begin{align}\nonumber
    & |\epsilon_\alpha(h)-\epsilon_t(h,y_t)| \\
    & = |\alpha \epsilon_e(h,\hat{y}_e)+(1-\alpha) \epsilon_h(h,\hat{y}_h)-\alpha \epsilon_e(h,y_e)-(1-\alpha)\epsilon_h(h,y_h)|\\
    & \le \alpha(|\epsilon_e(h,y_e)-\epsilon_h(h,y_h)|+|\epsilon_e(h,\hat{y}_e)-\epsilon_h(h,\hat{y}_h)|)+|\epsilon_h(h,\hat{y}_h)-\epsilon_h(h,y_h)|\\
    & = \alpha(\epsilon_a+\epsilon_b) + \epsilon_c
\end{align}

Then we seek the upper bound of $\epsilon_a,\epsilon_b,\epsilon_c$ by applying the triangle inequality for classification errors \citep{crammer2008learning} as stated in \textbf{Lemma 1}.
\begin{lemma}
For any hypotheses $f_1,f_2,f_3$ in class $\mathcal{H}$, 
\begin{equation}
    \epsilon(f_1,f_2) \le \epsilon(f_1,f_3)+\epsilon(f_2,f_3).
\end{equation}
\end{lemma}

For $\epsilon_a$, 
\begin{align}\nonumber
    & \epsilon_a=|\epsilon_e(h,y_e)-\epsilon_h(h,y_h)| \\
    & \le |\epsilon_e(h,y_e)-\epsilon_e(h,h^*)|+|\epsilon_e(h,h^*)-\epsilon_h(h,h^*)|+|\epsilon_h(h,h^*)-\epsilon_h(h,y_h)| \\
    & \le \epsilon_e(h^*)+|\epsilon_e(h,h^*)-\epsilon_h(h,h^*)|+\epsilon_h(h^*) \\
    & \le \frac{1}{2}d_{\mathcal{H}\triangle\mathcal{H}}(\mathcal{D}_e,\mathcal{D}_h)+\lambda
\end{align}

For $\epsilon_b$,
\begin{align}\nonumber
    & \epsilon_b=|\epsilon_e(h,\hat{y}_e)-\epsilon_h(h,\hat{y}_h)|\\
    & \le \epsilon_e(h^*,\hat{y}_e)+|\epsilon_e(h,h^*)-\epsilon_h(h,h^*)|+\epsilon_h(h^*,\hat{y}_h) \\
    & \le \frac{1}{2}d_{\mathcal{H}\triangle\mathcal{H}}(\mathcal{D}_c,\mathcal{D}_n)+(\epsilon_e(h^*,\hat{y}_e)+\epsilon_h(h^*,\hat{y}_h)) \\
    & \le \frac{1}{2}d_{\mathcal{H}\triangle\mathcal{H}}(\mathcal{D}_e,\mathcal{D}_h)+\hat{\lambda} \\
\end{align}

For $\epsilon_c$,
\begin{align}\nonumber
    & \epsilon_c= |\epsilon_h(h,\hat{y}_h)-\epsilon_h(h,y_h)| \le |\epsilon_h(\hat{y}_h,y_h)| = \rho_h
\end{align}

By summarizing $\epsilon_a,\epsilon_b,\epsilon_c$, we yield the inequality in \textbf{Theorem 1}:
\begin{align}
    & |\epsilon_\alpha(h)-\epsilon_t(h,y_t)| \\
    & \le \alpha[(\frac{1}{2}d_{\mathcal{H}\triangle\mathcal{H}}(\mathcal{D}_e,\mathcal{D}_h)+\lambda)+(\frac{1}{2}d_{\mathcal{H}\triangle\mathcal{H}}(\mathcal{D}_e,\mathcal{D}_h) + \hat{\lambda})]+\rho_h \\
    & = \alpha(d_{\mathcal{H}\triangle\mathcal{H}}(\mathcal{D}_e,\mathcal{D}_h)+\lambda+\hat{\lambda})+\rho_h
\end{align}
$\square$

Furthermore, the pseudo risk is bounded by the ideal risk, the pseudo rate of the clean set $\rho_e$ and the noisy set $\rho_h$, derived as follows:
\begin{align}
    & \hat{\lambda}=\epsilon_e(h^*,\hat{y}_e)+\epsilon_h(h^*,\hat{y}_h) \\
    & \le (\epsilon_e(h^*,y_e)+\epsilon_e(y_e,\hat{y}_e))+(\epsilon_h(h^*,y_h)+\epsilon_h(y_h,\hat{y}_h)) \\
    & = \lambda + \epsilon_e(y_e,\hat{y}_e)+\epsilon_h(y_h,\hat{y}_h) \\
    & = \lambda + \rho_e+\rho_h
\end{align}
Given a constant $\lambda$, when the easy-to-adapt subdomain is mostly correct, i.e., $\rho_e \approx 0$, the pseudo risk is bounded by the pseudo rate of the noisy set $\rho_h$.

\section{Hyper-parameter Settings}
We show the hyper-parameters utilized in our experiments in Table~\ref{tab:hyparams}, including $\tau$ for domain division, $\alpha$ for MixUp, $\lambda_{mse}$ that controls the weight of $\mathcal{L}_{mse}$ and the sharpening factor $T$. In semi-supervised learning, to prevent the noisy samples to cause error accumulation, we set $\lambda_{mse}$ to be 0. The Mixup follows a Beta distribution with $\alpha=1.0$. The sharpening factor $T=0.5$. We use $\tau=0.8$ for Office-31 and Office-Home. In VisDA-17, since the model may not perform confidently for the large challenging dataset, we set $\tau=0.5$ to ensure sufficient samples in the easy-to-adapt subdomain. 
\input{tables/hyperparams}

\section{Convergence of Losses}
Figure~\ref{fig:convergence} shows the convergence of the losses of BETA during the training procedure. The adversarial loss keeps small since the two subdomains are all drawn from the same domain and thus the distribution divergence between the two subdomains should be small. The mutual information is maximized as shown in the curve of $\mathcal{L}_{mi}$. The semi-supervised loss $\mathcal{L}_{dd}$ fluctuates while decreasing since two networks utilize the subdomains obtained by each other for semi-supervised learning, which decreases error accumulation.

\begin{figure*}[h]
	\centering
	\includegraphics[width=0.5\textwidth]{figures/loss_convergence.pdf}
	\caption{The training procedure of the method.}
	\label{fig:convergence}
\end{figure*}

\section{Domain Division}
In Figure~\ref{fig:division}, we show the domain division results at the first epoch (after the warm-up) on Office-Home (Art$\to$Clipart). The three rows contain three categories: alarm clocks, candles, and TV (monitors). The domain shift is very large between \textit{Art} and \textit{Clipart}, and the source-only accuracy is only 44.1\%. Even so, the domain division module still accurately divides the clean easy-to-adapt subdomain and the hard-to-adapt subdomain. In the easy-to-adapt subdomain, the contours of objects are similar to those of the source domain, such as the alarm clock. The domain shift between the easy-to-adapt subdomain and the source domain is smaller, as shown in the candle samples with a black background. For the TV, the easy-to-adapt samples have very clear contours and are easy to recognize. In comparison, the hard-to-adapt subdomain is more challenging in terms of shape, color, and style. Our domain division strategy outputs an AUC of 0.814 for the binary classification of clean samples and noisy samples whose pseudo labels are generated by the source-only model, which enables the semi-supervised learning in BETA to be reasonable. During the training, the AUC keeps increasing to 0.828 and further mitigates the confirmation bias progressively.

\begin{figure}[tbp]
	\centering
	\subfigure[Source domain (Art)]{\includegraphics[width=0.95\textwidth, angle=0]{figures/src-subdomain.pdf}\label{fig:src-domain}}
	\subfigure[Easy-to-adapt subdomain (Clipart)]{\includegraphics[width=0.95\textwidth, angle=0]{figures/easy-subdomain.pdf}\label{fig:easy-subdomain}}
	\caption{The domain division results on Office-Home (Art$\to$Clipart).}\label{fig:division}
\end{figure}

\section{Codes and Datasets}
We have attached the codes in the supplementary materials. The \textit{README.md} introduces the two steps: (i) train a source-only model, and (ii) train the BETA using the hard predictions of the source-only model. The datasets should be prepared in the \textit{data} folder using the official websites and their licenses should be followed \citep{saenko2010adapting,venkateswara2017deep,peng2017visda}.
